# Supplementary material for: DenoDet V2: Phase-Amplitude Cross Denoising for SAR Object Detection
Source: arXiv:2508.09392 source file (2025-08-12)
Supplement: Supplementary file 1 [file appendix.tex]

\clearpage
\clearpage
\appendix
\section{Implementation Details} \label{appdendix:implementation details}
\paragraph{Training.}
For training \ourdino{}, \ourmae{}, and CLIP models, we closely follow the existing open-source codebases: the official DINOv2 and MAE repositories, and the MetaCLIP codebase which builds on top of the OpenCLIP codebase~\citep{cherti2023reproducible}.
We use Fully Sharded Data Parallel (FSDP)~\citep{zhao2023pytorch} for distributed training of larger models.

For \ourdino{} and CLIP pretraining, we follow the exact recipe and hyperparameters from the original paper for their largest model.
For MAE pretraining, we observe that training becomes more prone to divergence as model size increases. To mitigate this, we reduce the learning rate from 2.4e-3 to 1.6e-3 and extend the warmup period to 80K iterations.
Table~\ref{tab:training_config} provides a summary of the pretraining hyperparameters.

\begin{table}[h]
    \centering
    \small
    \vspace{-0.1cm}
    \setlength\tabcolsep{3pt} % Adjusting column spacing
    \begin{tabular}{lcccc}
    \toprule
    Model & Batch Size  & Learning Rate & Warmup \\
    \midrule
    \ourdino{} & 3072  & 3.5e-4 & 100K  \\
    \ourmae{} & 4096  & 1.6e-3 & 80K   \\
    CLIP & 32768  & 4e-4 & 2K \\
    \bottomrule
    \end{tabular}
    
    \vspace{-0.1cm}
    \captionsetup{font=footnotesize}
    \caption{\footnotesize \textbf{Hyperparameters for \ourdino{}, \ourmae{} and CLIP.}}
    \label{tab:training_config}
    \vspace{-0.1cm}
\end{table}

% \TODO{JC: I updated the MAE recipe.}
% \

\paragraph{VQA evaluation.}
For VQA evaluation, we follow \citet{tong2024cambrian, tong2024metamorph} and use Cambrian-Alignment data for MLP projector training and Cambrian-7M for MLP and LLM fine-tuning. We finetune on top of Llama-3 8B Instruct~\citep{llama3modelcard}. The vision encoder is frozen throughout finetuning. We excluded LAION~\citep{schuhmann2022laion} images from the Cambrian data to comply with safety standards. We first encode the images at the model's original input resolution using the pretrained vision encoder. Next, we extract features from the final encoder layer. Following prior approaches~\citep{tong2024cambrian, tong2024metamorph}, we then resize the resulting token sequence to a fixed length of 576 tokens through bilinear interpolation. This ensures consistency across evaluations despite variations in input image resolutions. We report configurations in \cref{tab:cambrian training}.

\begin{table*}[h]
\centering
    \small  % Reducing font size to fit table
    \setlength\tabcolsep{2pt} % Default value: 6pt
    \begin{adjustbox}{max width=\textwidth}
    \begin{tabular}{l|cc|ccc|ccc}
    
 \multicolumn{1}{c|}{Backbone} & \multicolumn{2}{c|}{Data} & \multicolumn{3}{c|}{Adapter} &  \multicolumn{3}{c}{Instruction Tuning}\\
\multicolumn{1}{c|}{LLM} & Adapter & Instruction Tuning &     LR & WD & BS & LR & WD & BS \\
      \hline
 Llama-3 8B Instruct& Cambrian Adapter Data &  Cambrian-7M & 1.00e-5 & 0.0 & 512 & 4.00e-5 & 0 & 512 \\
    \end{tabular}
    \end{adjustbox}
         \vspace{-1em}
\caption{\small \textbf{Hyperparameters for all VQA experiments.} We exclude LAION~\citep{schuhmann2022laion} from Cambrian data. 
}
\label{tab:cambrian training}
\end{table*}

\paragraph{Classic vision evaluation.}

We follow the evaluation procedure in DINOv2~\citep{oquab2023dinov2} for all classic vision evaluation: linear probe on ImageNet1k~\citep{deng2009imagenet}, ADE20K~\citep{zhou2019semantic}, and NYU Depth v2~\citep{silberman2012indoor}. For ImageNet-1k, we evaluate models with their pretrained image resolution; For ADE20K and NYU Depth v2, we use the settings from \citet{oquab2023dinov2}. For ADE20K, we follow DINOv2 and report the \textbf{linear} and \textbf{+ms} setting. For NYU Depth v2, we report \textbf{lin. 1} and \textbf{lin. 4}. See the original paper for additional details.

\paragraph{Model architectures.}
In \cref{tab:vit config}, we defined the ViT architectures used in our study. To recap, we first borrowed the ViT-g architecture from~\citet{oquab2023dinov2} and named it ViT-1B for consistent notation. We then define 2B, 3B, 5B, and 7B architectures inspired by language model scaling. Specifically, the 2 - 7B architectures are wider than the 1B variant, inspired by language model recipes. Our 7B architecture is almost identical to the Llama-2 7B design, except for the patch embedding layer which is unique to ViTs.

\paragraph{Text filtering.}
In Question~\ref{rq:probe into text}, we introduced the ``Light'' and ``Heavy'' filters which retain 50.3\% and 1.3\% of \ourdata{} respectively. Specifically, we use a small MLLM, SmolVLM2~\citep{allal2025smollm2}, to identify images containing text, using prompts such as \textit{``Does this image contain any readable text?''}. The intention is not to achieve perfect filtering, but rather to skew the data distribution in the general desired direction. See \cref{fig:filter text} for a visualization of the filtering process and some examples. This results in two curated datasets:

(i) Light filter: Retains 50.3\% of the original data, primarily consisting of images with some textual content. Prompt used: \textit{``Does this image contain any readable text? Answer only yes or no.''}

(ii) Heavy filter: Retains only 1.3\% of the data, focusing mainly on charts and documents. Prompt used: \textit{``Please think carefully before answering. Does this image contain charts, tables, or documents with readable text? Answer only yes or no.''}

\section{Full Results} \label{appendix:full results}

We include full results of all experiments presented in \cref{sec:exp} and \cref{sec:analysis}. 

\subsection{\ourdino{}}

\paragraph{Scaling up model sizes.} We show quantitative results of scaling up the model under VQA evaluation in \cref{tab:VQA PIN-DINO MC-2B Data-2B} and classic vision evaluation in \cref{tab:Vision PIN-DINO MC-2B Data-2B}. These are the numerical results for \cref{subsec:scale vit}.

\begin{table*}[ht]
\centering
    \small  % Reducing font size to fit table
    \setlength\tabcolsep{2pt} % Default value: 6pt
    \begin{adjustbox}{max width=\textwidth}
    \begin{tabular}{l|r|rrrr|rrrr|rrrr|rrrr}
     \multicolumn{1}{c|}{Vision Backbone} &  \multicolumn{1}{c|}{} & \multicolumn{4}{c|}{General} & \multicolumn{4}{c|}{Knowledge} & \multicolumn{4}{c|}{OCR \& Chart} & \multicolumn{4}{c}{Vision-Centric}  \\
      Model  & \multicolumn{1}{c|}{\rotatebox{90}{Average}} & \multicolumn{1}{c}{\rotatebox{90}{MME$^\text{P}$}} & \multicolumn{1}{c}{\rotatebox{90}{MMB}} & \multicolumn{1}{c}{\rotatebox{90}{SEED$^\text{I}$}} & \multicolumn{1}{c|}{\rotatebox{90}{GQA}} & \multicolumn{1}{c}{\rotatebox{90}{SQA$^\text{I}$}} & \multicolumn{1}{c}{\rotatebox{90}{MMMU$^\text{V}$}} & \multicolumn{1}{c}{\rotatebox{90}{MathVista$^\text{M}$}} & \multicolumn{1}{c|}{\rotatebox{90}{AI2D}} & \multicolumn{1}{c}{\rotatebox{90}{ChartQA}} & \multicolumn{1}{c}{\rotatebox{90}{OCRBench}} & \multicolumn{1}{c}{\rotatebox{90}{TextVQA}} & \multicolumn{1}{c|}{\rotatebox{90}{DocVQA}} & \multicolumn{1}{c}{\rotatebox{90}{MMVP}} & \multicolumn{1}{c}{\rotatebox{90}{RealWorldQA}} & \multicolumn{1}{c}{\rotatebox{90}{CV-Bench$^\text{2D}$}} & \multicolumn{1}{c}{\rotatebox{90}{CV-Bench$^\text{3D}$}} \\
\hline 
% \rowcolor{gray!10} \multicolumn{2}{l|}{Language-Supervised}  &  &  &  &  &  &  &  &  &  &  &  &  &  &  &  & & \\
\ourdino{} ViT-1B & 49.01 & 1731.52 & 65.37 & 69.92 & 62.40 & 72.58 & 35.33 & 12.30 & 64.28 & 19.20 & 9.40 & 47.41 & 17.00 & 37.33 & 57.12 & 64.80 & 63.16 \\
\ourdino{} ViT-2B & 50.77 & 1760.80 & 68.98 & 71.29 & 62.89 & 73.67 & 31.77 & 15.90 & 67.06 & 23.30 & 15.60 & 49.20 & 19.00 & 38.00 & 57.38 & 65.85 & 64.41\\
\ourdino{} ViT-3B & 51.71 & 1757.27 & 68.04 & 71.84 & 63.19 & 73.57 & 33.00 & 14.40 & 67.32 & 25.68 & 17.10 & 50.45 & 20.00 & 42.66 & 56.86 & 69.49 & 65.83 \\
\ourdino{} ViT-5B & 52.83 & 1840.81 & 70.01 & 72.39 & 63.56 & 75.06 & 32.11 & 12.40 & 67.77 & 26.96 & 22.10 & 50.64 & 21.00 & 44.66 & 57.64 & 67.75 & 69.16 \\
\ourdino{} ViT-7B & 53.87 & 1823.76 & 68.98 & 73.02 & 64.22 & 74.61 & 35.11 & 14.00 & 69.43 & 28.80 & 23.59 & 51.10 & 22.00 & 48.00 & 59.34 & 69.96 & 68.58
    \end{tabular}
\end{adjustbox}
\caption{\textbf{VQA Evaluation: \ourdino{} trained on \ourdata{} with 2 billion images seen.}}
\label{tab:VQA PIN-DINO MC-2B Data-2B}
\end{table*}

\begin{table*}[ht]
\centering
    \small  % Reducing font size to fit table
    \setlength\tabcolsep{6pt} % Adjusting column spacing
    \begin{adjustbox}{max width=\textwidth}
    \begin{tabular}{l|ccccc}
     \multicolumn{1}{c|}{Vision Backbone} & \multicolumn{1}{c}{\rotatebox{0}{IN1k lin.}} & \multicolumn{1}{c}{\rotatebox{0}{ADE20K lin.}} & \multicolumn{1}{c}{\rotatebox{0}{ADE20K +ms.}} & \multicolumn{1}{c}{\rotatebox{0}{NYUd lin. 1 (↓)} } & \multicolumn{1}{c}{\rotatebox{0}{NYUd lin. 4 (↓)}} \\
\hline 
\ourdino{} ViT-1B & 84.70 & 46.60 & 50.97 & 0.364 & 0.345 \\
\ourdino{} ViT-2B & 85.16 & 50.55 & 52.32 & 0.351 & 0.335 \\
\ourdino{} ViT-3B & 85.66 & 50.17 & 53.12 & 0.348 & 0.328 \\
\ourdino{} ViT-5B & 85.84 & 49.54 & 53.27 & 0.378 & 0.335 \\
\ourdino{} ViT-7B & 86.00 & 49.08 & 54.65 & 0.380 & 0.339 \\
    \end{tabular}
\end{adjustbox}
\caption{\textbf{Classic Vision Evaluation: \ourdino{} trained on \ourdata{} with 2 billion images seen.}}
\label{tab:Vision PIN-DINO MC-2B Data-2B}
\end{table*}

\paragraph{Scaling up data sizes.} We show quantitative results of scaling up the number of data seen with \ourdino{} ViT-7B on VQA evaluation in \cref{tab:VQA PIN-DINO MC-2B Data-scale} and classic vision evaluation in \cref{tab:Vision PIN-DINO MC-2B Data-scale}. These are the numerical results for \cref{subsec:scale data}.

\begin{table*}[ht]
\centering
    \small  % Reducing font size to fit table
    \setlength\tabcolsep{2pt} % Default value: 6pt
    \begin{adjustbox}{max width=\textwidth}
    \begin{tabular}{l|r|rrrr|rrrr|rrrr|rrrr}
     \multicolumn{1}{c|}{Vision Backbone} &  \multicolumn{1}{c|}{} & \multicolumn{4}{c|}{General} & \multicolumn{4}{c|}{Knowledge} & \multicolumn{4}{c|}{OCR \& Chart} & \multicolumn{4}{c}{Vision-Centric}  \\
      Model  & \multicolumn{1}{c|}{\rotatebox{90}{Average}} & \multicolumn{1}{c}{\rotatebox{90}{MME$^\text{P}$}} & \multicolumn{1}{c}{\rotatebox{90}{MMB}} & \multicolumn{1}{c}{\rotatebox{90}{SEED$^\text{I}$}} & \multicolumn{1}{c|}{\rotatebox{90}{GQA}} & \multicolumn{1}{c}{\rotatebox{90}{SQA$^\text{I}$}} & \multicolumn{1}{c}{\rotatebox{90}{MMMU$^\text{V}$}} & \multicolumn{1}{c}{\rotatebox{90}{MathVista$^\text{M}$}} & \multicolumn{1}{c|}{\rotatebox{90}{AI2D}} & \multicolumn{1}{c}{\rotatebox{90}{ChartQA}} & \multicolumn{1}{c}{\rotatebox{90}{OCRBench}} & \multicolumn{1}{c}{\rotatebox{90}{TextVQA}} & \multicolumn{1}{c|}{\rotatebox{90}{DocVQA}} & \multicolumn{1}{c}{\rotatebox{90}{MMVP}} & \multicolumn{1}{c}{\rotatebox{90}{RealWorldQA}} & \multicolumn{1}{c}{\rotatebox{90}{CV-Bench$^\text{2D}$}} & \multicolumn{1}{c}{\rotatebox{90}{CV-Bench$^\text{3D}$}} \\
\hline 
% \rowcolor{gray!10} \multicolumn{2}{l|}{Language-Supervised}  &  &  &  &  &  &  &  &  &  &  &  &  &  &  &  & & \\
\ourdino{} ViT-7B (1B Data) & 51.02 & 1785.97 & 68.12 & 72.54 & 63.60 & 73.87 & 32.88 & 12.70 & 66.58 & 23.60 & 15.20 & 49.04 & 19.00 & 43.33 & 57.12 & 68.35 & 61.08 \\
\ourdino{} ViT-7B (2B Data) & 53.87 & 1823.76 & 68.98 & 73.02 & 64.22 & 74.61 & 35.11 & 14.00 & 69.43 & 28.80 & 23.59 & 51.10 & 22.00 & 48.00 & 59.34 & 69.96 & 68.58 \\
\ourdino{} ViT-7B (4B Data) & 54.37 & 1827.12 & 71.39 & 72.61 & 63.53 & 72.73 & 34.00 & 18.90 & 67.09 & 35.12 & 30.00 & 53.19 & 24.00 & 45.33 & 55.94 & 69.68 & 65.00\\
\ourdino{} ViT-7B (8B Data) & 55.24 & 1811.05 & 71.30 & 72.14 & 64.04 & 72.43 & 35.66 & 15.20 & 68.52 & 35.52 & 36.40 & 56.53 & 29.00 & 46.00 & 57.90 & 70.53 & 62.08 \\
% \ourdino{} ViT-7B (8B Data) & 56.04 & 1815.09 & 69.84 & 72.33 & 63.96 & 75.55 & 33.33 & 13.50 & 68.84 & 46.76 & 35.90 & 57.51 & 36.00 & 43.33 & 58.03 & 70.29 & 60.75 \\

    \end{tabular}
\end{adjustbox}
\caption{\textbf{VQA Evaluation: \ourdino{} ViT-7B trained on \ourdata{} with increased number of images seen.}}
\label{tab:VQA PIN-DINO MC-2B Data-scale}
\end{table*}

\begin{table*}[ht]
\centering
    \small  % Reducing font size to fit table
    \setlength\tabcolsep{6pt} % Adjusting column spacing
    \begin{adjustbox}{max width=\textwidth}
    \begin{tabular}{l|ccccc}
     \multicolumn{1}{c|}{Vision Backbone} & \multicolumn{1}{c}{\rotatebox{0}{IN1k lin.}} & \multicolumn{1}{c}{\rotatebox{0}{ADE20K lin.}} & \multicolumn{1}{c}{\rotatebox{0}{ADE20K +ms.}} & \multicolumn{1}{c}{\rotatebox{0}{NYUd lin. 1 (↓)} } & \multicolumn{1}{c}{\rotatebox{0}{NYUd lin. 4 (↓)}} \\
\hline 
\ourdino{} ViT-7B (2B Data) & 86.00 & 49.08 & 54.65 & 0.380 & 0.339 \\
\ourdino{} ViT-7B (4B Data) & 86.33 & 47.41 & 54.66 & 0.416 & 0.363 \\
\ourdino{} ViT-7B (8B Data) & 86.52 & 42.14 & 52.55 & 0.491 & 0.376 \\
    \end{tabular}
\end{adjustbox}
\caption{\textbf{Classic Vision Evaluation: \ourdino{} ViT-7B trained on \ourdata{} with increased number of images seen.}}
\label{tab:Vision PIN-DINO MC-2B Data-scale}
\end{table*}

\paragraph{Scaling down training data.} We show VQA evaluation results from training \ourdino{} on less diverse data--ImageNet-1k, in \cref{tab:VQA PIN-DINO ImageNet Data-scale}. These are the full results for scaling down training data experiments in  Question~\ref{rq:small data}.

\begin{table*}[ht]
\centering
    \small  % Reducing font size to fit table
    \setlength\tabcolsep{2pt} % Default value: 6pt
    \begin{adjustbox}{max width=\textwidth}
    \begin{tabular}{l|r|rrrr|rrrr|rrrr|rrrr}
     \multicolumn{1}{c|}{Vision Backbone} &  \multicolumn{1}{c|}{} & \multicolumn{4}{c|}{General} & \multicolumn{4}{c|}{Knowledge} & \multicolumn{4}{c|}{OCR \& Chart} & \multicolumn{4}{c}{Vision-Centric}  \\
      Model  & \multicolumn{1}{c|}{\rotatebox{90}{Average}} & \multicolumn{1}{c}{\rotatebox{90}{MME$^\text{P}$}} & \multicolumn{1}{c}{\rotatebox{90}{MMB}} & \multicolumn{1}{c}{\rotatebox{90}{SEED$^\text{I}$}} & \multicolumn{1}{c|}{\rotatebox{90}{GQA}} & \multicolumn{1}{c}{\rotatebox{90}{SQA$^\text{I}$}} & \multicolumn{1}{c}{\rotatebox{90}{MMMU$^\text{V}$}} & \multicolumn{1}{c}{\rotatebox{90}{MathVista$^\text{M}$}} & \multicolumn{1}{c|}{\rotatebox{90}{AI2D}} & \multicolumn{1}{c}{\rotatebox{90}{ChartQA}} & \multicolumn{1}{c}{\rotatebox{90}{OCRBench}} & \multicolumn{1}{c}{\rotatebox{90}{TextVQA}} & \multicolumn{1}{c|}{\rotatebox{90}{DocVQA}} & \multicolumn{1}{c}{\rotatebox{90}{MMVP}} & \multicolumn{1}{c}{\rotatebox{90}{RealWorldQA}} & \multicolumn{1}{c}{\rotatebox{90}{CV-Bench$^\text{2D}$}} & \multicolumn{1}{c}{\rotatebox{90}{CV-Bench$^\text{3D}$}} \\
\hline 
% \rowcolor{gray!10} \multicolumn{2}{l|}{Language-Supervised}  &  &  &  &  &  &  &  &  &  &  &  &  &  &  &  & & \\
\ourdino{} ViT-1B & 46.39 & 1704.30 & 59.27 & 66.43 & 60.12 & 71.29 & 32.77 & 18.70 & 63.40 & 17.56 & 4.90 & 44.93 & 14.00 & 32.00 & 52.41 & 62.81 & 56.41
 \\
\ourdino{} ViT-2B & 45.99 & 1666.01 & 60.13 & 66.64 & 60.19 & 68.71 & 34.88 & 12.10 & 62.07 & 18.60 & 4.39 & 45.55 & 14.00 & 32.66 & 52.67 & 62.07 & 57.83 \\
\ourdino{} ViT-3B & 46.43 & 1729.40 & 60.56 & 66.99 & 60.24 & 70.50 & 31.88 & 11.70 & 62.30 & 17.52 & 4.80 & 45.18 & 15.00 & 31.33 & 53.20 & 62.77 & 62.50 \\
\ourdino{} ViT-5B & 46.28 & 1661.25 & 59.27 & 67.24 & 61.10 & 69.41 & 31.55 & 10.90 & 61.46 & 18.72 & 4.60 & 45.53 & 15.00 & 34.00 & 53.07 & 64.57 & 61.08 \\

    \end{tabular}
\end{adjustbox}
\caption{\textbf{VQA Evaluation: \ourdino{} trained on ImageNet-1k.}}
\label{tab:VQA PIN-DINO ImageNet Data-scale}
\end{table*}

\subsection{\ourmae{}}

We show VQA evaluation results from scaling up MAE trained on \ourdata{}, in \cref{tab:VQA PIN-MAE MC-2B}. These are the full results for Question~\ref{rq:generalize to other ssl}.

\begin{table*}[ht]
\centering
    \small  % Reducing font size to fit table
    \setlength\tabcolsep{2pt} % Default value: 6pt
    \begin{adjustbox}{max width=\textwidth}
    \begin{tabular}{l|r|rrrr|rrrr|rrrr|rrrr}
     \multicolumn{1}{c|}{Vision Backbone} &  \multicolumn{1}{c|}{} & \multicolumn{4}{c|}{General} & \multicolumn{4}{c|}{Knowledge} & \multicolumn{4}{c|}{OCR \& Chart} & \multicolumn{4}{c}{Vision-Centric}  \\
      Model  & \multicolumn{1}{c|}{\rotatebox{90}{Average}} & \multicolumn{1}{c}{\rotatebox{90}{MME$^\text{P}$}} & \multicolumn{1}{c}{\rotatebox{90}{MMB}} & \multicolumn{1}{c}{\rotatebox{90}{SEED$^\text{I}$}} & \multicolumn{1}{c|}{\rotatebox{90}{GQA}} & \multicolumn{1}{c}{\rotatebox{90}{SQA$^\text{I}$}} & \multicolumn{1}{c}{\rotatebox{90}{MMMU$^\text{V}$}} & \multicolumn{1}{c}{\rotatebox{90}{MathVista$^\text{M}$}} & \multicolumn{1}{c|}{\rotatebox{90}{AI2D}} & \multicolumn{1}{c}{\rotatebox{90}{ChartQA}} & \multicolumn{1}{c}{\rotatebox{90}{OCRBench}} & \multicolumn{1}{c}{\rotatebox{90}{TextVQA}} & \multicolumn{1}{c|}{\rotatebox{90}{DocVQA}} & \multicolumn{1}{c}{\rotatebox{90}{MMVP}} & \multicolumn{1}{c}{\rotatebox{90}{RealWorldQA}} & \multicolumn{1}{c}{\rotatebox{90}{CV-Bench$^\text{2D}$}} & \multicolumn{1}{c}{\rotatebox{90}{CV-Bench$^\text{3D}$}} \\
\hline 
% \rowcolor{gray!10} \multicolumn{2}{l|}{Language-Supervised}  &  &  &  &  &  &  &  &  &  &  &  &  &  &  &  & & \\
\ourmae{} ViT-1B & 49.19 & 1736.22 & 62.02 & 68.38 & 60.05 & 73.27 & 33.11 & 12.90 & 63.92 & 23.60 & 16.40 & 47.84 & 18.00 & 36.66 & 52.81 & 70.42 & 60.83

 \\
\ourmae{} ViT-2B & 50.59 & 1700.16 & 63.57 & 69.21 & 60.93 & 72.48 & 32.22 & 15.50 & 64.44 & 29.00 & 23.20 & 48.78 & 20.00 & 38.00 & 55.16 & 67.98 & 63.91
\\
\ourmae{} ViT-3B & 50.92 & 1723.85 & 64.69 & 69.71 & 60.94 & 72.13 & 34.33 & 13.50 & 65.70 & 30.92 & 24.60 & 48.92 & 20.00 & 37.33 & 54.64 & 64.15 & 66.91
 \\
\ourmae{} ViT-5B & 51.50 & 1710.13 & 65.12 & 70.13 & 61.10 & 72.63 & 32.66 & 13.90 & 65.67 & 33.80 & 26.50 & 49.60 & 21.00 & 38.00 & 53.72 & 66.69 & 67.91
 \\

    \end{tabular}
\end{adjustbox}
\caption{\textbf{VQA Evaluation: \ourmae{} trained on \ourdata{}.}}
\label{tab:VQA PIN-MAE MC-2B}
\end{table*}

\subsection{Scaled CLIP Models}

We show VQA evaluation results from scaling up  MetaCLIP~\citep{xu2023demystifying} trained on \ourdata{}, in \cref{tab:VQA CLIP MC-2B}. These are the full results for \cref{subsec:scale vit}. In contrast to visual SSL methods in \cref{tab:Vision PIN-DINO MC-2B Data-2B} and \cref{tab:VQA PIN-MAE MC-2B}, CLIP models do not exhibit clear scaling behavior.

\begin{table*}[ht]
\centering
    \small  % Reducing font size to fit table
    \setlength\tabcolsep{2pt} % Default value: 6pt
    \begin{adjustbox}{max width=\textwidth}
    \begin{tabular}{l|r|rrrr|rrrr|rrrr|rrrr}
     \multicolumn{1}{c|}{Vision Backbone} &  \multicolumn{1}{c|}{} & \multicolumn{4}{c|}{General} & \multicolumn{4}{c|}{Knowledge} & \multicolumn{4}{c|}{OCR \& Chart} & \multicolumn{4}{c}{Vision-Centric}  \\
      Model  & \multicolumn{1}{c|}{\rotatebox{90}{Average}} & \multicolumn{1}{c}{\rotatebox{90}{MME$^\text{P}$}} & \multicolumn{1}{c}{\rotatebox{90}{MMB}} & \multicolumn{1}{c}{\rotatebox{90}{SEED$^\text{I}$}} & \multicolumn{1}{c|}{\rotatebox{90}{GQA}} & \multicolumn{1}{c}{\rotatebox{90}{SQA$^\text{I}$}} & \multicolumn{1}{c}{\rotatebox{90}{MMMU$^\text{V}$}} & \multicolumn{1}{c}{\rotatebox{90}{MathVista$^\text{M}$}} & \multicolumn{1}{c|}{\rotatebox{90}{AI2D}} & \multicolumn{1}{c}{\rotatebox{90}{ChartQA}} & \multicolumn{1}{c}{\rotatebox{90}{OCRBench}} & \multicolumn{1}{c}{\rotatebox{90}{TextVQA}} & \multicolumn{1}{c|}{\rotatebox{90}{DocVQA}} & \multicolumn{1}{c}{\rotatebox{90}{MMVP}} & \multicolumn{1}{c}{\rotatebox{90}{RealWorldQA}} & \multicolumn{1}{c}{\rotatebox{90}{CV-Bench$^\text{2D}$}} & \multicolumn{1}{c}{\rotatebox{90}{CV-Bench$^\text{3D}$}} \\
\hline 
MetaCLIP ViT-1B & 52.30 & 1813.70 & 68.90 & 69.45 & 60.35 & 74.07 & 33.55 & 12.70 & 64.41 & 33.20 & 34.59 & 52.15 & 26.00 & 37.33 & 52.15 & 65.47 & 61.83
 \\
MetaCLIP ViT-2B & 53.03 & 1787.39 & 68.81 & 69.54 & 61.08 & 75.16 & 34.66 & 20.10 & 65.38 & 32.80 & 32.90 & 52.55 & 26.00 & 37.33 & 52.94 & 65.19 & 64.67
\\
MetaCLIP ViT-3B & 53.22 & 1873.67 & 68.72 & 70.33 & 61.85 & 77.29 & 32.77 & 11.80 & 66.35 & 32.16 & 34.40 & 54.58 & 26.00 & 35.33 & 55.55 & 65.57 & 65.08
 \\
MetaCLIP ViT-5B & 52.52 & 1779.03 & 70.10 & 70.26 & 61.53 & 72.43 & 33.44 & 17.90 & 66.74 & 30.04 & 32.20 & 52.49 & 25.00 & 39.33 & 54.50 & 64.22 & 61.16
 \\
MetaCLIP ViT-7B & 52.97 & 1827.80 & 69.93 & 69.47 & 61.33 & 74.91 & 35.55 & 16.80 & 65.15 & 32.12 & 32.10 & 52.07 & 25.00 & 39.33 & 54.11 & 65.08 & 63.16

 \\

    \end{tabular}
\end{adjustbox}
\caption{\textbf{VQA Evaluation: MetaCLIP trained on \ourdata{} with 2 billion images seen.}}
\label{tab:VQA CLIP MC-2B}
\end{table*}

\subsection{Text Filtered Models}
We provide full results for Question~\ref{rq:probe into text}. As shown in \cref{tab:VQA MC-DINO Text Filterd Models}, SSL models learn features particularly well-suited for OCR \& Chart tasks when trained on datasets with a higher concentration of text-rich images. This suggests that visual SSL is sensitive to the underlying training distribution and can be effectively steered toward specific downstream applications, such as OCR \& Chart.
\begin{table*}[ht]
\centering
    \small  % Reducing font size to fit table
    \setlength\tabcolsep{2pt} % Default value: 6pt
    \begin{adjustbox}{max width=\textwidth}
    \begin{tabular}{l|r|rrrr|rrrr|rrrr|rrrr}
     \multicolumn{1}{c|}{Vision Backbone} &  \multicolumn{1}{c|}{} & \multicolumn{4}{c|}{General} & \multicolumn{4}{c|}{Knowledge} & \multicolumn{4}{c|}{OCR \& Chart} & \multicolumn{4}{c}{Vision-Centric}  \\
      Model  & \multicolumn{1}{c|}{\rotatebox{90}{Average}} & \multicolumn{1}{c}{\rotatebox{90}{MME$^\text{P}$}} & \multicolumn{1}{c}{\rotatebox{90}{MMB}} & \multicolumn{1}{c}{\rotatebox{90}{SEED$^\text{I}$}} & \multicolumn{1}{c|}{\rotatebox{90}{GQA}} & \multicolumn{1}{c}{\rotatebox{90}{SQA$^\text{I}$}} & \multicolumn{1}{c}{\rotatebox{90}{MMMU$^\text{V}$}} & \multicolumn{1}{c}{\rotatebox{90}{MathVista$^\text{M}$}} & \multicolumn{1}{c|}{\rotatebox{90}{AI2D}} & \multicolumn{1}{c}{\rotatebox{90}{ChartQA}} & \multicolumn{1}{c}{\rotatebox{90}{OCRBench}} & \multicolumn{1}{c}{\rotatebox{90}{TextVQA}} & \multicolumn{1}{c|}{\rotatebox{90}{DocVQA}} & \multicolumn{1}{c}{\rotatebox{90}{MMVP}} & \multicolumn{1}{c}{\rotatebox{90}{RealWorldQA}} & \multicolumn{1}{c}{\rotatebox{90}{CV-Bench$^\text{2D}$}} & \multicolumn{1}{c}{\rotatebox{90}{CV-Bench$^\text{3D}$}} \\
\hline 
\textcolor{gray}{\ourdino{} ViT-1B (No Filter)} & \textcolor{gray}{49.01} & \textcolor{gray}{1731.52} & \textcolor{gray}{65.37} & \textcolor{gray}{69.92} & \textcolor{gray}{62.40} & \textcolor{gray}{72.58} & \textcolor{gray}{35.33} & \textcolor{gray}{12.30} & \textcolor{gray}{64.28} & \textcolor{gray}{19.20} & \textcolor{gray}{9.40} & \textcolor{gray}{47.41} & \textcolor{gray}{17.00} & \textcolor{gray}{37.33} & \textcolor{gray}{57.12} & \textcolor{gray}{64.80} & \textcolor{gray}{63.16} \\

\ourdino{} ViT-1B (Light Filter) & 50.73 & 1690.89 & 65.54 & 70.68 & 62.63 & 70.99 & 33.89 & 17.80 & 63.69 & 26.12 & 21.80 & 50.56 & 20.00 & 36.00 & 56.86 & 64.84 & 65.75 \\

\ourdino{} ViT-1B (Heavy Filter) & 49.44 & 1593.79 & 61.40 & 65.34 & 59.53 & 71.19 & 31.33 & 14.90 & 64.83 & 36.92 & 24.09 & 50.09 & 27.00 & 21.33 & 53.20 & 66.53 & 63.66
 \\
\textcolor{gray}{\ourdino{} ViT-2B (No Filter)} & \textcolor{gray}{50.77} & \textcolor{gray}{1760.80} & \textcolor{gray}{68.98} & \textcolor{gray}{71.29} & \textcolor{gray}{62.89} & \textcolor{gray}{73.67} & \textcolor{gray}{31.77} & \textcolor{gray}{15.90} & \textcolor{gray}{67.06} & \textcolor{gray}{23.30} & \textcolor{gray}{15.60} & \textcolor{gray}{49.20} & \textcolor{gray}{19.00} & \textcolor{gray}{38.00} & \textcolor{gray}{57.38} & \textcolor{gray}{65.85} & \textcolor{gray}{64.41} \\
\ourdino{} ViT-2B (Light Filter) & 53.38 & 1768.67 & 68.38 & 71.80 & 63.24 & 74.16 & 33.88 & 31.40 & 67.38 & 31.40 & 27.30 & 51.26 & 23.00 & 39.33 & 56.47 & 61.13 & 65.50

 \\
\ourdino{} ViT-2B (Heavy Filter) & 53.65 & 1743.56 & 65.29 & 69.28 & 61.19 & 74.86 & 32.22 & 14.50 & 67.42 & 47.48 & 29.40 & 52.80 & 32.00 & 40.00 & 54.50 & 65.85 & 64.50

    \end{tabular}
\end{adjustbox}
\caption{\textbf{VQA Evaluation: \ourdino{} trained on text filtered \ourdata{}.}}
\label{tab:VQA MC-DINO Text Filterd Models}
\end{table*}

\subsection{Baseline Models}
In \cref{tab:VQA Reference Models}, we provide full VQA results for the reference off-shelf models that we evaluated in \cref{sec:final model}. 

\begin{table*}[ht]
\centering
    \small  % Reducing font size to fit table
    \setlength\tabcolsep{2pt} % Default value: 6pt
    \begin{adjustbox}{max width=\textwidth}
    \begin{tabular}{l|r|rrrr|rrrr|rrrr|rrrr}
     \multicolumn{1}{c|}{Vision Backbone} &  \multicolumn{1}{c|}{} & \multicolumn{4}{c|}{General} & \multicolumn{4}{c|}{Knowledge} & \multicolumn{4}{c|}{OCR \& Chart} & \multicolumn{4}{c}{Vision-Centric}  \\
      Model  & \multicolumn{1}{c|}{\rotatebox{90}{Average}} & \multicolumn{1}{c}{\rotatebox{90}{MME$^\text{P}$}} & \multicolumn{1}{c}{\rotatebox{90}{MMB}} & \multicolumn{1}{c}{\rotatebox{90}{SEED$^\text{I}$}} & \multicolumn{1}{c|}{\rotatebox{90}{GQA}} & \multicolumn{1}{c}{\rotatebox{90}{SQA$^\text{I}$}} & \multicolumn{1}{c}{\rotatebox{90}{MMMU$^\text{V}$}} & \multicolumn{1}{c}{\rotatebox{90}{MathVista$^\text{M}$}} & \multicolumn{1}{c|}{\rotatebox{90}{AI2D}} & \multicolumn{1}{c}{\rotatebox{90}{ChartQA}} & \multicolumn{1}{c}{\rotatebox{90}{OCRBench}} & \multicolumn{1}{c}{\rotatebox{90}{TextVQA}} & \multicolumn{1}{c|}{\rotatebox{90}{DocVQA}} & \multicolumn{1}{c}{\rotatebox{90}{MMVP}} & \multicolumn{1}{c}{\rotatebox{90}{RealWorldQA}} & \multicolumn{1}{c}{\rotatebox{90}{CV-Bench$^\text{2D}$}} & \multicolumn{1}{c}{\rotatebox{90}{CV-Bench$^\text{3D}$}} \\
\hline 
\rowcolor{gray!10} CLIP Models    &  &  &  &  &  &  &   &  &  & &  &  & & &  &  & 
\\
MetaCLIP ViT-H$_{224\text{px}}$ & 54.91 & 1860.58 & 72.93 & 70.96 & 62.22 & 77.88 & 36.88 & 15.00 & 67.32 & 35.60 & 33.40 & 55.10 & 29.00 & 41.33 & 53.46 & 68.53 & 65.91 \\
SigLIP ViT-SO400M$_{224\text{px}}$ & 55.36 & 1807.30 & 72.76 & 71.83 & 62.68 & 76.74 & 35.44 & 14.00 & 68.65 & 33.08 & 40.20 & 56.61 & 28.00 & 47.33 & 56.99 & 66.42 & 64.66 
 \\
SigLIP ViT-SO400M$_{384\text{px}}$ & 59.97 & 1892.16 & 73.71 & 73.00 & 63.80 & 77.83 & 33.88 & 20.00 & 69.78 & 54.24 & 46.40 & 63.53 & 50.00 & 46.00 & 58.43 & 67.37 & 66.91

 \\

SigLIP2 ViT-SO400M$_{224\text{px}}$ & 56.32 & 1789.26 & 73.36 & 72.20 & 62.60 & 74.96 & 35.55 & 22.40 & 69.85 & 35.76 & 42.00 & 59.68 & 31.00 & 44.00 & 54.24 & 69.88 & 64.16
\\

SigLIP2 ViT-SO400M$_{384\text{px}}$ & 61.98 & 1895.70 & 74.57 & 72.24 & 64.81 & 79.27 & 36.33 & 19.90 & 72.24 & 59.68 & 52.90 & 67.15 & 54.00 & 49.33 & 54.77 & 70.73 & 69.00

\\

\rowcolor{gray!10}SSL Models    &  &  &  &  &  &  &   &  &  & &  &  & & &  &  & 
\\
DINOv2 ViT-g$_{224\text{px}}$  & 49.25 & 1785.25 & 64.86 & 70.89 & 62.89 & 72.03 & 32.11 & 12.40 & 62.37 & 17.96 & 5.50 & 47.06 & 15.00 & 47.33 & 56.33 & 65.92 & 66.08
\\

DINOv2 ViT-g$_{378\text{px}}$ & 47.94 & 1734.38 & 64.26 & 71.50 & 62.21 & 71.04 & 33.11 & 9.60 & 63.08 & 17.76 & 5.00 & 45.59 & 15.00 & 41.33 & 56.47 & 63.79 & 60.58

\\

DINOv2 ViT-g$_{518\text{px}}$ & 47.91 & 1694.08 & 62.45 & 70.64 & 62.87 & 71.29 & 33.55 & 11.80 & 63.37 & 18.32 & 5.10 & 46.27 & 15.00 & 37.33 & 56.60 & 65.36 & 61.83

\\
I-JEPA ViT-H $_{224\text{px}}$ & 44.78 & 1598.15 & 60.01 & 64.04 & 57.66 & 68.91 & 34.55 & 10.20 & 62.07 & 16.72 & 4.00 & 42.99 & 14.00 & 29.33 & 49.93 & 57.39 & 57.16

 \\
MAE ViT-H$_{224\text{px}}$ & 45.21 & 1697.06 & 56.87 & 56.41 & 60.51 & 70.74 & 32.11 & 11.50 & 61.30 & 17.40 & 5.50 & 45.38 & 14.00 & 27.33 & 53.46 & 61.19 & 64.75

 \\

    \end{tabular}
\end{adjustbox}
\caption{\textbf{VQA Evaluation: Off-shelf CLIP and SSL models.}}
\label{tab:VQA Reference Models}
\end{table*}

\section{High Resolution Adaption of \ourssl{}}
\label{appendix:high res}
Following \citet{oquab2023dinov2}, we further fine-tune our model under higher resolution settings of 378$\times$378 and 518$\times$518 for 20k iterations. We use a batch size of 2048 and a correspondingly lower learning rate of 1.41e-5. All other parameters remain exactly the same as previously specified, including the learning rate warmup ratio, given the total of 10k iterations.

We also provided detailed benchmark results of high-resolution adaptation of \ourdino{} in \cref{tab:Our Highres Models}.

\begin{table*}[ht]
\centering
    \small  % Reducing font size to fit table
    \setlength\tabcolsep{2pt} % Default value: 6pt
    \begin{adjustbox}{max width=\textwidth}
    \begin{tabular}{l|r|rrrr|rrrr|rrrr|rrrr}
     \multicolumn{1}{c|}{Vision Backbone} &  \multicolumn{1}{c|}{} & \multicolumn{4}{c|}{General} & \multicolumn{4}{c|}{Knowledge} & \multicolumn{4}{c|}{OCR \& Chart} & \multicolumn{4}{c}{Vision-Centric}  \\
      Model  & \multicolumn{1}{c|}{\rotatebox{90}{Average}} & \multicolumn{1}{c}{\rotatebox{90}{MME$^\text{P}$}} & \multicolumn{1}{c}{\rotatebox{90}{MMB}} & \multicolumn{1}{c}{\rotatebox{90}{SEED$^\text{I}$}} & \multicolumn{1}{c|}{\rotatebox{90}{GQA}} & \multicolumn{1}{c}{\rotatebox{90}{SQA$^\text{I}$}} & \multicolumn{1}{c}{\rotatebox{90}{MMMU$^\text{V}$}} & \multicolumn{1}{c}{\rotatebox{90}{MathVista$^\text{M}$}} & \multicolumn{1}{c|}{\rotatebox{90}{AI2D}} & \multicolumn{1}{c}{\rotatebox{90}{ChartQA}} & \multicolumn{1}{c}{\rotatebox{90}{OCRBench}} & \multicolumn{1}{c}{\rotatebox{90}{TextVQA}} & \multicolumn{1}{c|}{\rotatebox{90}{DocVQA}} & \multicolumn{1}{c}{\rotatebox{90}{MMVP}} & \multicolumn{1}{c}{\rotatebox{90}{RealWorldQA}} & \multicolumn{1}{c}{\rotatebox{90}{CV-Bench$^\text{2D}$}} & \multicolumn{1}{c}{\rotatebox{90}{CV-Bench$^\text{3D}$}} \\
\hline

\ourdino{}$_{224\text{px}}$ &  55.24 & 1811.05 & 71.30 & 72.14 & 64.04 & 72.43 & 35.66 & 15.20 & 68.52 & 35.52 & 36.40 & 56.53 & 29.00 & 46.00 & 57.90 & 70.53 & 62.08

\\
\ourdino{}$_{378\text{px}}$ & 57.43 & 1757.06 & 70.61 & 72.59 & 64.50 & 72.53 & 35.11 & 16.10 & 67.09 & 52.04 & 42.19 & 61.51 & 46.00 & 38.00 & 59.08 & 66.55 & 67.16

\\
\ourdino{}$_{518\text{px}}$ &  59.91 & 1807.08 & 73.79 & 72.92 & 64.78 & 74.36 & 34.66 & 14.50 & 69.43 & 57.28 & 45.70 & 64.48 & 53.00 & 43.33 & 60.52 & 70.08 & 69.41

    \end{tabular}
\end{adjustbox}
\caption{\textbf{VQA Evaluation: \ourdino{} ViT-7B adapted to different resolution}}
\label{tab:Our Highres Models}
\end{table*}

\section{Evaluation}

\cref{tab:benchmarks} lists evaluation benchmarks used and their purposes.

\begin{table}[htbp]
\centering
\begin{tabular}{lll}
\hline
Benchmark & Eval & Citation \\
\hline
GQA & General VQA & \citet{hudson2019gqa} \\
SEED & General VQA & \citet{ge2023planting} \\
MME & General VQA & \citet{fu2023mme} \\
MMBench & General VQA & \citet{liu2023mmbench} \\

AI2D & Knowledge VQA & \citet{hiippala2021ai2d} \\
ScienceQA & Knowledge VQA & \citet{lu2022learn} \\
MathVista & Knowledge VQA & \citet{lu2023mathvista} \\
MMMU & Knowledge VQA & \citet{yue2023mmmu} \\

TextVQA & OCR \& Chart VQA & \citet{singh2019towards} \\
DocVQA & OCR \& Chart VQA & \citet{mathew2021docvqa} \\
ChartQA & OCR \& Chart VQA & \citet{masry2022chartqa} \\
OCRBench & OCR \& Chart VQA & \citet{liu2023hidden} \\

MMVP & Vision-Centric VQA & \citet{tong2024eyes} \\
RealWorldQA & Vision-Centric VQA & \citet{grok} \\
CVBench-2D & Vision-Centric VQA & \citet{tong2024cambrian} \\
CVBench-3D & Vision-Centric VQA & \citet{tong2024cambrian} \\
ImageNet-1k & Image Classification & \citet{deng2009imagenet} \\
ADE-20k & Image Segmentation &\citet{zhou2019semantic} \\
NYU Depth v2 & Depth Estimation & \citet{silberman2012indoor} \\

\hline
\end{tabular}
\caption{\textbf{List of benchmarks used}}
\label{tab:benchmarks}
\end{table}

\section{Pretraining Dataset Cards}
\label{appendix:pretrain_dataset}
For reference, in \cref{tab:lvd_data_statistics} we include the data composition of LVD-142M, which was used to train the off-shelf DINOv2 model~\citep{oquab2023dinov2}. LVD-142M is a carefully curated data mix closely aligned with downstream classic vision evaluation tasks.
In comparison, we leverage MetaCLIP data, which is less curated and collected from 15 snapshots of CommonCrawl (CC).

\begin{table*}
\centering
\footnotesize
\begin{tabular}{lllrrr}
\hline
Task & Dataset / Split & Images & Retrieval & Retrieved & Final \\
\hline
classification & ImageNet-22k / -- & 14,197,086 & as is & -- & 14,197,086 \\
classification & ImageNet-22k / -- & 14,197,086 & sample & 56,788,344 & 56,788,344 \\
classification & ImageNet-1k / train & 1,281,167 & sample & 40,997,344 & 40,997,344 \\
\hline
fine-grained classif. & Caltech 101 / train & 3,030 & cluster & 2,630,000 & 1,000,000 \\
fine-grained classif. & CUB-200-2011 / train & 5,994 & cluster & 1,300,000 & 1,000,000 \\
fine-grained classif. & DTD / train1 & 1,880 & cluster & 1,580,000 & 1,000,000 \\
fine-grained classif. & FGVC-Aircraft / train & 3,334 & cluster & 1,170,000 & 1,000,000 \\
fine-grained classif. & Flowers-102 / train & 1,020 & cluster & 1,060,000 & 1,000,000 \\
fine-grained classif. & Food-101 / train & 75,750 & cluster & 21,670,000 & 1,000,000 \\
fine-grained classif. & Oxford-IIIT Pet / trainval & 3,680 & cluster & 2,750,000 & 1,000,000 \\
fine-grained classif. & Stanford Cars / train & 8,144 & cluster & 7,220,000 & 1,000,000 \\
fine-grained classif. & SUN397 / train1 & 19,850 & cluster & 18,950,000 & 1,000,000 \\
fine-grained classif. & Pascal VOC 2007 / train & 2,501 & cluster & 1,010,000 & 1,000,000 \\
\hline
segmentation & ADE20K / train & 20,210 & cluster & 20,720,000 & 1,000,000 \\
segmentation & Cityscapes / train & 2,975 & cluster & 1,390,000 & 1,000,000 \\
segmentation & Pascal VOC 2012 (seg.) / trainaug & 1,464 & cluster & 10,140,000 & 1,000,000 \\
\hline
depth estimation & Mapillary SLS / train & 1,434,262 & as is & -- & 1,434,262 \\
depth estimation & KITTI / train (Eigen) & 23,158 & cluster & 3,700,000 & 1,000,000 \\
depth estimation & NYU Depth V2 / train & 24,231 & cluster & 10,850,000 & 1,000,000 \\
depth estimation & SUN RGB-D / train & 4,829 & cluster & 4,870,000 & 1,000,000 \\
\hline
retrieval & Google Landmarks v2 / train (clean) & 1,580,470 & as is & -- & 1,580,470 \\
retrieval & Google Landmarks v2 / train (clean) & 1,580,470 & sample & 6,321,880 & 6,321,880 \\
retrieval & AmsterTime / new & 1,231 & cluster & 960,000 & 960,000 \\
retrieval & AmsterTime / old & 1,231 & cluster & 830,000 & 830,000 \\
retrieval & Met / train & 397,121 & cluster & 62,860,000 & 1,000,000 \\
retrieval & Revisiting Oxford / base & 4,993 & cluster & 3,680,000 & 1,000,000 \\
retrieval & Revisiting Paris / base & 6,322 & cluster & 3,660,000 & 1,000,000 \\
\hline
&&&&&142,109,386 \\
\hline
\end{tabular}
\caption{\textbf{LVD-142M Data Sources.} In contrast to LVD-142M, which relies on highly curated data sources drawn from distributions closely aligned with various downstream evaluation tasks (see the table above from \citet{oquab2023dinov2}), our data curation approach adopts the methodology from MetaCLIP~\citep{xu2023demystifying}, utilizing web data collected from 15 snapshots of CommonCrawl (CC) spanning January 2021 through January 2023.}
\label{tab:lvd_data_statistics}

\end{table*}
